# Supplementary material for: Sparse Visual Thought Circuits in Vision-Language Models
Source: arXiv:2603.25075 source file (2026-03-26)
Supplement: Supplementary file 1 [file heldout_supp_valtest_key_configs.tex]

\begin{tabular}{llrlll}
\toprule
Split & Config & scale & ΔAcc(pp) & P(Δ>0) & Changed(%) \\
\midrule
val & pattern & 2.000000 & +0.50 $\pm$ 0.46 & 0.60 & 10.50 $\pm$ 0.90 \\
val & pattern_plus_global & 0.500000 & -1.30 $\pm$ 0.73 & 0.00 & 16.23 $\pm$ 0.92 \\
val & global & 0.500000 & +0.20 $\pm$ 0.88 & 0.60 & 13.53 $\pm$ 0.56 \\
test & pattern & 2.000000 & +0.37 $\pm$ 0.61 & 0.60 & 11.43 $\pm$ 1.62 \\
test & pattern_plus_global & 0.500000 & -1.00 $\pm$ 0.60 & 0.00 & 14.90 $\pm$ 1.19 \\
test & global & 0.500000 & +0.03 $\pm$ 0.58 & 0.20 & 13.63 $\pm$ 1.10 \\
\bottomrule
\end{tabular}
