# Supplementary material for: Sparse Visual Thought Circuits in Vision-Language Models
Source: arXiv:2603.25075 source file (2026-03-26)
Supplement: Supplementary file 2 [file p0_combo_per_label_bootstrap.tex]

\begin{tabular}{lcccc}
\toprule
Task type & Pattern ($2\times$) & Global ($0.5\times$) & Union ($2\times$) & Union ($0.5\times$) \\
\midrule
spatial & +1.10 $\pm$ 1.05 & +1.75 $\pm$ 1.54 & -6.36 $\pm$ 2.25 & +0.78 $\pm$ 1.42 \\
counting & +0.64 $\pm$ 1.46 & -0.38 $\pm$ 0.34 & +5.70 $\pm$ 2.24 & -0.12 $\pm$ 0.53 \\
existence & +0.00 $\pm$ 0.00 & +0.00 $\pm$ 0.00 & -1.20 $\pm$ 1.10 & +0.00 $\pm$ 0.00 \\
pattern & +3.96 $\pm$ 1.52 & +4.96 $\pm$ 3.91 & -1.90 $\pm$ 1.51 & -1.44 $\pm$ 1.81 \\
comparison & +1.49 $\pm$ 1.27 & -1.42 $\pm$ 2.65 & -5.09 $\pm$ 3.73 & -2.70 $\pm$ 1.57 \\
attribute_logic & -0.88 $\pm$ 2.49 & -5.71 $\pm$ 3.87 & +0.81 $\pm$ 2.88 & -5.27 $\pm$ 3.16 \\
global & -0.34 $\pm$ 0.77 & +4.49 $\pm$ 2.08 & -1.91 $\pm$ 2.31 & +2.43 $\pm$ 1.89 \\
\bottomrule
\end{tabular}
