# Supplementary material for: Sparse Visual Thought Circuits in Vision-Language Models
Source: arXiv:2603.25075 source file (2026-03-26)
Supplement: Supplementary file 3 [file targeted_vs_random_summary.tex]

\begin{tabular}{llcccc}
\toprule
Set & Config & $\Delta$Acc (pp) & $P(\Delta>0)$ & Changed (\%) & Runs \\
\midrule
Targeted & pattern, scale 2.0 & +1.03 $\pm$ 0.66 & 1.00 & 10.97 $\pm$ 1.58 & 5 \\
Targeted & global, scale 0.5 & +0.57 $\pm$ 0.88 & 0.80 & 13.07 $\pm$ 1.92 & 5 \\
\midrule
Random & pattern, scale 2.0 & +0.17 $\pm$ 0.00 & 1.00 & 13.94 $\pm$ 0.19 & 3 \\
Random & global, scale 0.5 & +0.17 $\pm$ 0.00 & 1.00 & 13.67 $\pm$ 0.29 & 3 \\
\bottomrule
\end{tabular}
